# Supplementary material for: Coherent exciton-exciton interactions and exciton dynamics in a MoSe\textsubscript{2}/WSe\textsubscript{2} heterostructure
Source: arXiv:2106.03739 ancillary file (2021-06-07)
Supplement: Supplementary file 1 [file HS_Dynamics_SI_v1.pdf]

# Coherent exciton-exciton interactions and exciton dynamics in a $MoSe_2/WSe_2$ heterostructure - Supplementary information

Torben L. Purz,[1] Eric. W. Martin,[1,2] Pasqual Rivera,[3] William G. Holtzmann,[3] Xiaodong Xu,[3] and Steven T. Cundiff[1,*]

[1] *University of Michigan, Department of Physics, Ann Arbor, MI, USA*
[2] *MONSTR Sense Technologies, LLC, Ann Arbor, MI, USA*
[3] *Department of Physics, University of Washington, Seattle, WA, USA*

(Dated: May 26, 2021)

## SAMPLE PREPARATION

The sample consists of mechanically exfoliated $MoSe_2$ and $WSe_2$ monolayers stacked on top of each other with a near-zero twist angle. The heterostructure is encapsulated in hexagonal boron nitride (hBN) and contains thin graphite layers on top and bottom. The sample was assembled using a dry-transfer technique with a stamp made of a polydimethylsiloxane cylinder with a thin film of poly(bisphenol A carbonate) on top.

## EXPERIMENTAL SETUP AND MDCS SCHEME

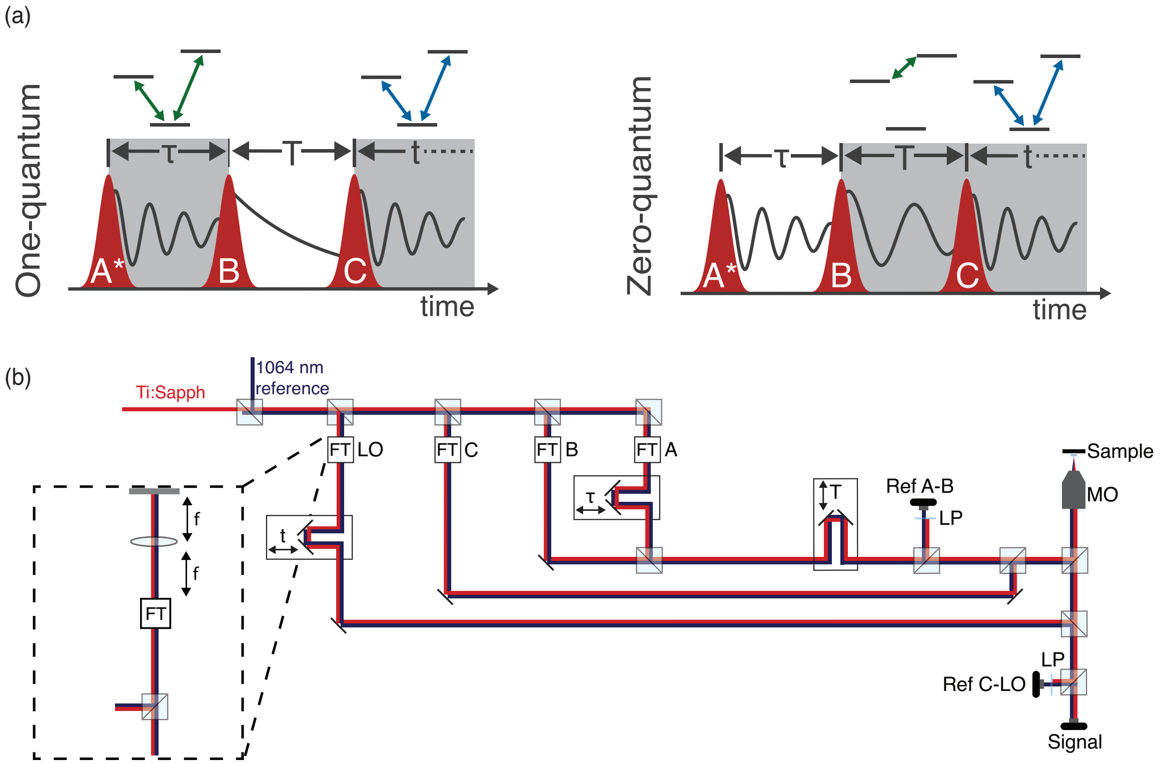


FIG. S1. **a** Scheme for one-quantum MDCS. The system is in a coherence during $\tau$ and $t$, which are scanned and Fourier transformed. **b** Scheme for one-quantum MDCS. The system is in a Raman-like coherence between the excited states during $T$, whose Fourier transform yields the mixing energy. **c** Schematic drawing of the MDCS setup used to obtain the data presented in the main text and SI.

* cundiff@umich.edu

The MDCS scheme and experimental setup are shown in Fig. S1. The sample is cooled to 5 K using an Advanced Research Systems (ARS) closed cycle cryostat. Pulses from the Coherent Vitara laser (30 fs transform limited, centered at 1660 meV) coming into the setup are chirp pre-compensated to durations $< 100$ fs at the sample using a homebuilt Grism compressor. Beams are frequency-tagged using acousto-optics modulators (Isomet 1205-C). The recombined beams (0.2 pJ/beam) are subsequently focused onto the sample using a long working distance Nikon 20x, NA=0.4 objective (1 $\mu$m spot diameter). The three beams and four-wave mixing are subsequently interfered with a local oscillator (LO) and detected on a silicon variable gain detector (New Focus, Model 2031). The detected signal is sent to a lock-in amplifier (MONSTR Sense Technologies). All four beams are co-propagated by a 50 mW, 1064 nm Nd:Yag Laser (CrystaLaser) which references path length changes between A-B and C-D. The signal from this reference is used to calculate the FWM reference for lock-in detection. For the zero-quantum spectrum in Fig. 3 (b), we block beam B and send the frequency shifts for A and B to the A AOM in order to use the higher resolution $\tau$ stage for the zero-quantum scan. This also ensures perfect temporal overlap of the A and B (pump) excitations.

Intentional chirp, used to study the coherent coupling, is applied onto the pulses by varying the Grism separation in the Grism compressor.

## Low-temperature PL measurements

Low-temperature optical PL measurements were performed at 5 K inside of a closed cycle cryostat (Montana Instruments Cryostation C2) using a HeNe laser (632.8 nm) for excitation, focused to a 1 µm spot diameter. A power of 100 µW was used for the PL presented in this paper. A 90/10 beamsplitter transmitted the collected PL, which was subsequently passed through a longpass filter and polarization optics. PL measurements presented in this work used right-handed circular (R) excitation and left-handed circular (L) detection. The PL was detected using a spectrometer (Princeton Instruments Acton 500 mm) and a liquid-nitrogen-cooled silicon-based CCD array. The grating used had 600 grooves per mm.

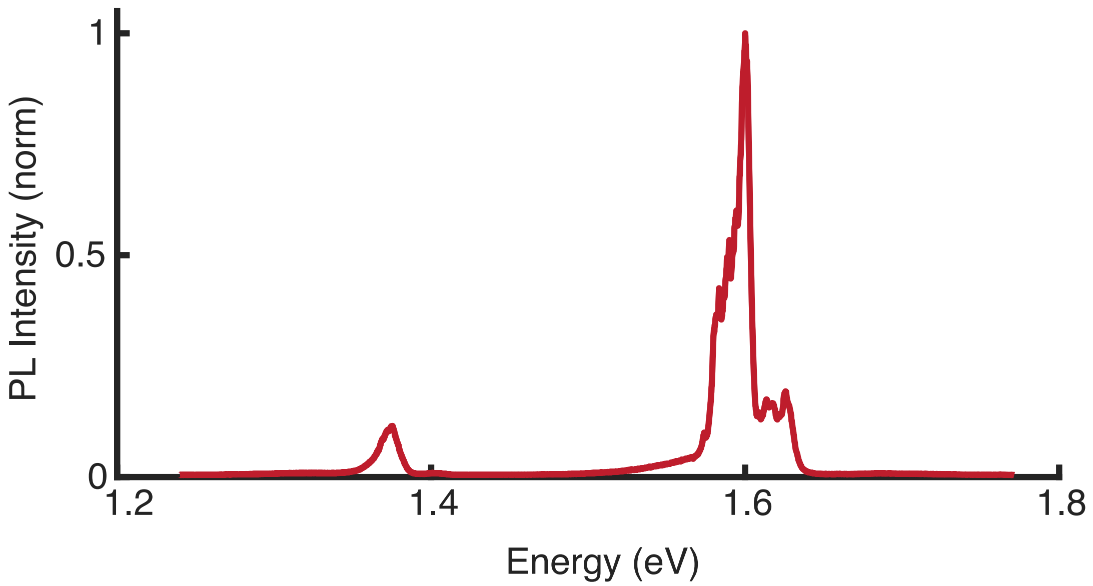


FIG. S2. Full energy range PL spectrum of the $MoSe_2/WSe_2$ heterostructure with right-circular polarized excitation and left-circular polarized detection.

Fig. S2 shows the full energy range photoluminescence (PL) spectrum of the heterostructure sample, taken with a HeNe laser power of 100 $\mu$W. The $MoSe_2$ A-exciton peak can clearly be seen around 1.6 eV, as shown in the main text the $WSe_2$ peak is significantly weaker. The interlayer exciton emission appears at an energy of 1.37 meV, which is used in the main text to calculate the interlayer exciton binding energy.

## LINEWIDTH FITS

Fig. S3 (a) shows a rephasing spectrum for the heterostructure. The rephasing spectrum shows significantly broadened peaks compared to the rephasing and non-rephasing spectra added in the main text. This is further amplified due to the normalization of the rephasing spectrum by the laser spectrum, which enhances the wings of the spectrum. Since it is not essential to the effects observed in the main text and tends to increase noise, we only normalize the rephasing spectrum here with this procedure to get a more accurate picture for the linewidths.

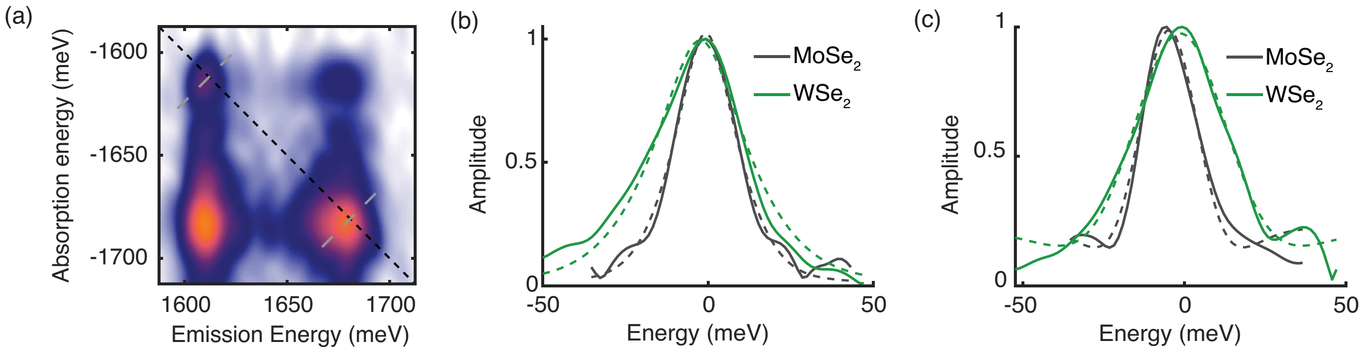


FIG. S3. **a** Rephasing spectrum for the $MoSe_2/WSe_2$ heterostructure **b** Cross diagonal slices (light gray dashed line in (a)) for the $MoSe_2$ and $WSe_2$ peak with corresponding fits with a Voigt profile (dashed lines). **c** On-diagonal slices for the $MoSe_2$ and $WSe_2$ peak with corresponding fits with a Voigt profile (dashed lines).

The rephasing spectrum allows us to extract homogeneous and inhomogeneous linewidths according to the procedure outlined in [1] by fitting the cross-diagonal (gray dashed line in Fig. S3 (a)) and on-diagonal slices (black dashed line in Fig. S3 (a)) simultaneously. The cross-diagonal slices are plotted in Fig. S3 (b), the on-diagonal slices are plotted in Fig. S3 (c). As outlined in [1], we fit the slices with a Voigt profile to obtain quantitative information about the homogeneous and inhomogeneous linewidths. The fits are indicated by the dashed lines in Fig. S3 (b,c). We extract the homogeneous linewidths $\gamma_{\mathrm{MoSe_2}}$=8.5 meV, $\gamma_{\mathrm{WSe_2}}$=16.9 meV, and inhomogeneous linewidths $\sigma_{\mathrm{MoSe_2}}$=11.7 meV, $\sigma_{\mathrm{WSe_2}}$=20.8 meV. While the fits are not well constrained due to the edges of the peaks being at the outer wings of the spectrum, as well as peak overlap limitations, they still give a good estimate of the homogeneous and inhomogeneous linewidths within a factor of 1-2 and show a clear increase of the homogeneous linewidth compared to the literature, which has seen instrinsic (zero-temperature, zero-power) homogeneous linewidths of 0.26 meV for $MoSe_2$ [2] and 1.6 meV for $WSe_2$ [3]. The latter measurement was performed on a CVD grown sample in a non-collinear geometry, substantially increasing the spot size at the sample. While we cannot extract an instrinsic linewidth due to experimental limitations, the power, and temperature dependent data the authors provide in their respective publications indicate that our intrinsic linewidth should at best be 2-3 times smaller than the values above, still showing a significant increase for the linewidths in the heterostructure compared to the monolayers.

## TEMPORAL RESOLUTION

We derive an estimate for the temporal resolution of our technique using the method outlined in [4]. This work notes that absorption profiles narrower than the pulse bandwidth have an effectively higher temporal resolution than what the chirp-limited pulse duration might initially suggest. In Fig. S4(a) we plot the pulse profile at the sample that has been characterized via cross-correlation. In Fig. S4(b) we plot the assumed absorption profile for the $MoSe_2$ and $WSe_2$ resonance on the heterostructure, estimated from the MDCS spectra. Since we are only interested in a rough estimate of our temporal resolution, this is sufficient. In Fig. S4 (c) we plot the corresponding temporal response function for the on-diagonal $MoSe_2$ and $WSe_2$ peak, as well as the two coupling peaks according to the procedure outlined in [4]. This plot shows the pump-probe signal for an instantaneous response. We generalize the procedure of [4] by using the sample absorption(which also corresponds to the emission) of the two resonances in both the preparation and observation window. Using the $MoSe_2$ absorption for both the preparation and observation window, we obtain the temporal profile for the $MoSe_2$ peak in Fig. S4. Similarly, we obtain the temporal profile for the $WSe_2$ peak. We obtain the profile for the coupling peak by assuming absorption from one resonance for the preparation, and absorption from the other resonance in the observation window. The symmetry of the expression in [4] automatically leads to the same temporal resolution for both coupling peaks. We then estimate the temporal resolution from the

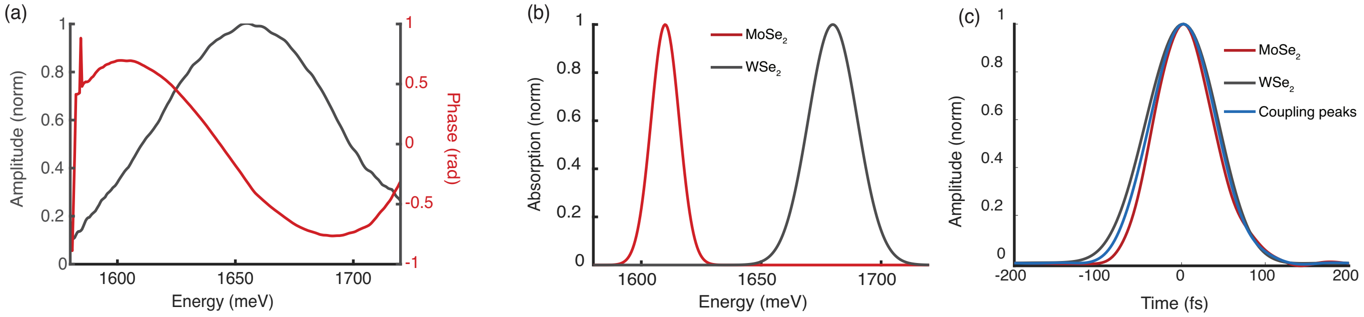


FIG. S4. **a** Temporal profile (amplitude and phase) of the pulse at the sample, characterized via cross-correlation. **b** Approximated absorption profile on the heterostructure for $MoSe_2$ and $WSe_2$. **c** Temporal intensity profile of the on-diagonal and coupling peak response assuming an instantaneous sample response and the absorption profile shown in (a).

full-width-half-maximum (FWHM) of the displayed temporal intensity profiles, which read 83 fs for the $MoSe_2$ peak, 100 fs for the $WSe_2$ peak, and 92 fs for the coupling peaks. This procedure does not account for possible offsets along $T$ for the two coupling peaks, however it gives a resolution estimate on the exponential fits for the charge transfer time.

## SIMPLE MODELS FOR COHERENT AND INCOHERENT COUPLING

In Fig. S5 we show the two underlying level systems for incoherent coupling via charge transfer (Fig. S5(a)) and coherent coupling between the $MoSe_2$ and $WSe_2$ excitons (Fig. S5(b)). For the case of incoherent coupling, the $MoSe_2$ and $WSe_2$ excitons generally have separate ground states. While this level system can explain the occurrence of coupling peaks due to population transfer, no oscillatory signal during $T$ occurs in this case. Instead, as discussed in the main text, the coupling peaks will experience a rise with a time-scale characteristic of the charge transfer in this case due to the electrons and holes affecting the absorption and exciton properties of the monolayers (see also [5]).

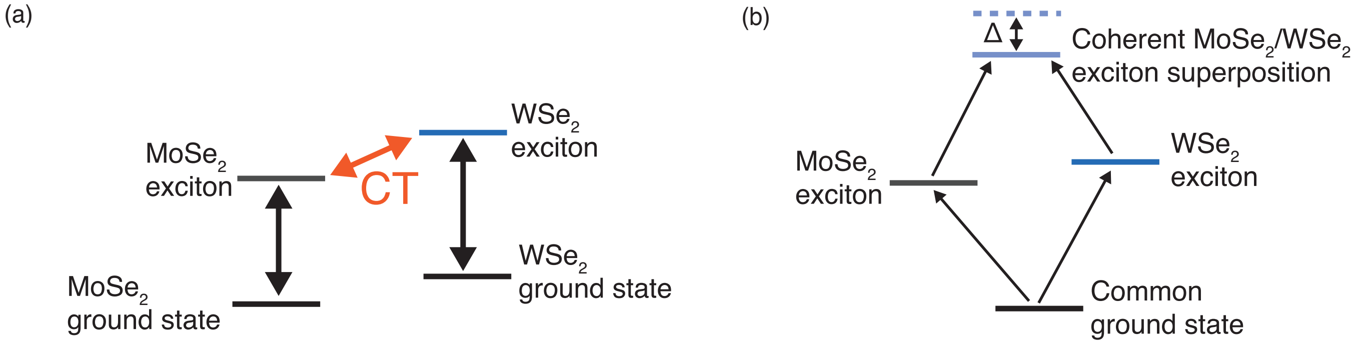


FIG. S5. **a** Two separate two-level systems for $MoSe_2$ and $WSe_2$ in the case of incoherent coupling via charge transfer. **b** Diamond level system in the case of coherent coupling between $MoSe_2$ and $WSe_2$.

In the case of coherent coupling, displayed in Fig. S5(b), it is easier to use a diamond energy level system with the $MoSe_2$ and $WSe_2$ exciton sharing a common ground state and forming a doubly excited state. The diamond system is obtained by taking the outer product of the Hilbert spaces for the individual two level systems. If there are no interactions, the "new" signal pathways, i.e., those that did not exist for two separate two-level systems, perfectly cancel. However if there are interactions, which result in a change in the energy, dephasing or dipole moment, for the singly to doubly excited transitions compared to the ground to singly excited states, then the cancellation is incomplete and new signals occur. For simplicity, we have only drawn the V-level system part of the diamond system in the main text, which is valid if interactions are sufficiently strong. The V-level system has an oscillating signal during $T$ whose frequency matches the energy difference between the $MoSe_2$ and $WSe_2$ excitons. This is not meant to be a detailed discussion of the level systems and processes contributing to shifts of energy levels. This picture is not complete since it does not contain the doubly-excited $MoSe_2$ or doubly-excited $WSe_2$ state. However it illustrates that, no matter the reason for the shift of the coherent superposition state, an oscillation with the correct frequency is

a strong indicator of coherent coupling. Future investigations using double-quantum spectroscopy could further shed light onto the dynamics of the coherent superposition and doubly-excited states and many-body interactions between the excitons.

Since we observe both coherent and incoherent (charge transfer) coupling in our sample, the energy diagram will correspond to the diamond level system shown in Fig. S5(b), with additional incoherent coupling between the $MoSe_2$ and $WSe_2$ excitons.

## CHIRP DEPENDENCE OF COHERENT COUPLING

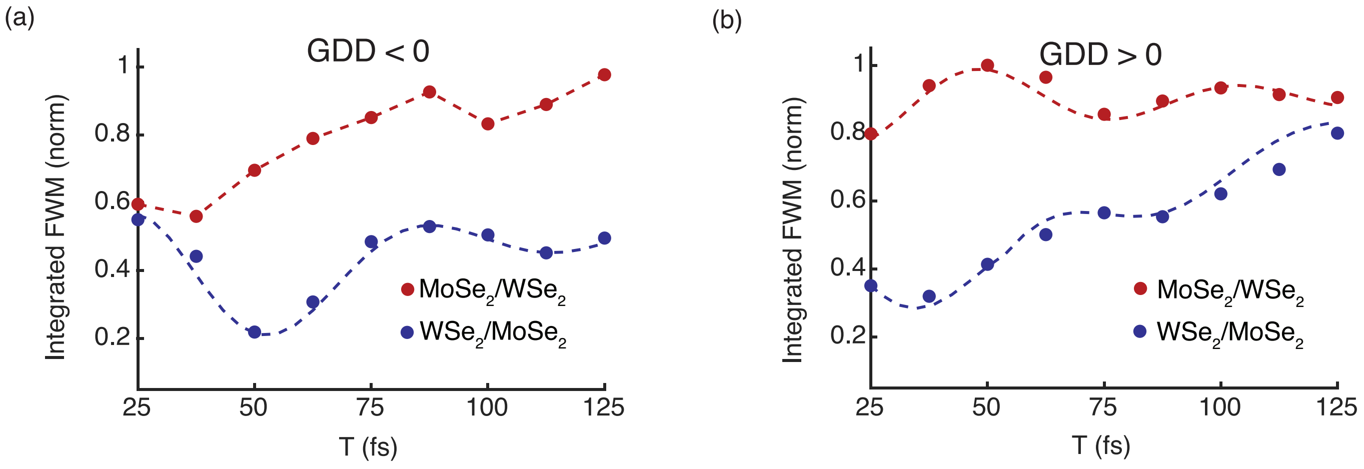


FIG. S6. Chirp dependence of the two coupling peak amplitudes in one-quantum spectra for **a** negative GDD and **b** positive GDD.

In the main text we present composite data for the peak oscillations and zero-quantum spectra with intentional positive and negative chirp. We apply this chirp by adjusting the grism distance in the Grism compressor. While this slightly affects the third-order dispersion, too, the effect is negligible here. In Fig. S6 (a,b) we present the full dataset for the coupling peak oscillations. As in the main text, the offset between the curves is chosen arbitrarily to enhance visibility. We also plot a decaying oscillation together with an exponential rise as a guide to the eye. Note that the time-zero for the exponential rise is adjusted for some of the guide to the eye curves presented here because the time-zero for transfer dynamics along $T$ is offset by the chirp. In Fig. S6 (a) we detuned the group-delay dispersion (GDD) to be negative. The oscillation on the $WSe_2/MoSe_2$ coupling peak can clearly be resolved, while the $MoSe_2/WSe2_2$ coupling peak only shows a weak oscillatory feature. Because of the chirp, the rise of the coupling peak has occured at what are negative $T$ times here and thus does not show up for the $WSe_2/MoSe_2$ coupling peak, while the peak rise is the dominant contribution for the $MoSe_2/WSe_2$ peak. In Fig. S6 (b) we detune the GDD to be positive. Here, the $MoSe_2/WSe_2$ peak has a clearly visible oscillation with no significant exponential rise, as explained above. Even the $WSe_2/MoSe_2$ shows a residual oscillation, although it is clearly obstructed by the rise behavior and not as pronounced as in Fig. S6 (a).

We similarly adjust the chirp for the zero-quantum spectra. The spectra provided in the main text are a summation of Fig. S7 (a), which shows the zero-quantum spectrum for negative GDD and Fig. S7 (c) which shows the zero quantum spectrum for positive GDD. We also show a zero intentional GDD (and thus limited by third order residual chirp) spectrum in Fig. S7 (b). Similarly to Fig. S6, we can resolve the coherent coupling from $WSe_2$ to $MoSe_2$ with intentional negative GDD in Fig. S7 (a) and the coherent coupling from $MoSe_2$ to $WSe_2$ with intentional positive GDD in Fig. S7 (c). The coherent coupling peaks occur at +71 meV and -74 meV respectively, matching the difference in the resonance energies between the two materials well as explained in the main text. For the positive GDD case, we have removed values below $T$=25 fs in the main text, which eliminates some spurious contributions at intermediate mixing energies. However, we did not remove the values here to simplify comparison with the simulations below. Even in the zero intentional GDD case, we can retain features reminiscent of the two coupling peaks. The broad features extending towards negative mixing energies for the $MoSe_2$ emission and towards positive mixing energies for the $WSe_2$ emission are reminiscent of the coherent coupling. They show up at lower mixing energies because only the edges of the broad resonances that are closer together in energy (and thus timing) contribute to these zero-quantum spectra.

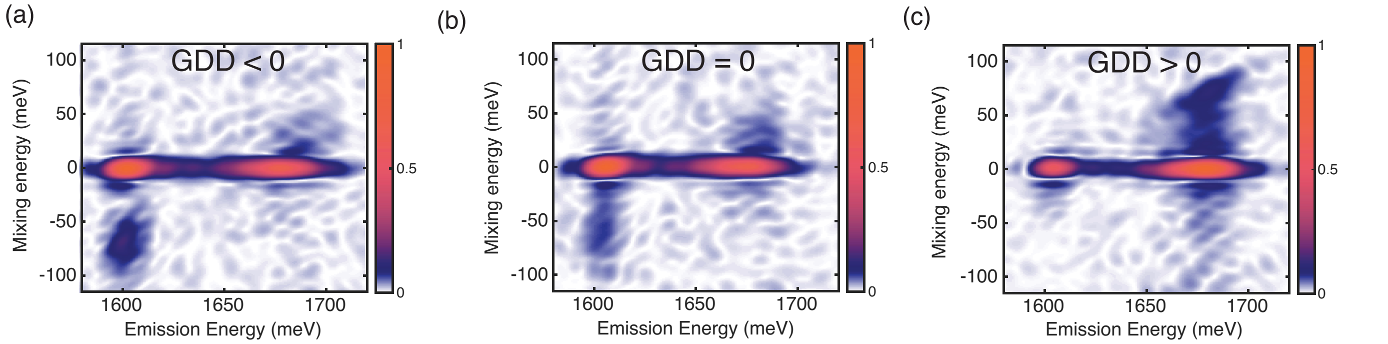


FIG. S7. Zero-quantum spectra in the presence of negative additional GDD (a), no intentional GDD, but residual TOD (b) and positive additional GDD (c). The coherent coupling between $MoSe_2$ and $WSe2_2$ can clearly be resolved for negative and positive intentional GDD.

To get a better justification of the intentional chirp scheme, we perform simulations of the optical Bloch equations (OBEs) using the measured spectral amplitude and phase of our pulse. In the simplest case, the OBEs, which are the equations of motion for the matrix elements of the density operator $\rho$ read [6]

$$\dot{\rho}_{ij} = -\frac{i}{\hbar}\sum_{k}\left(H_{ik}\rho_{kj} - \rho_{ik}H_{kj}\right) - \gamma_{ij}\rho_{ij}. \quad (1)$$

| $\gamma_{0M}$ | $\gamma_{0W}$ | $\gamma_{MW}$ | $\gamma_{MM}$ | $E_M$ | $E_W$ | $\mu_{0M}/\mu_{0W}$ | $E_0$ |
|---|---|---|---|---|---|---|---|
| 12.5 $ps^{-1}$ | 20 $ps^{-1}$ | 6.67 $ps^{-1}$ | 20 $ps^{-1}$ | 1610 meV | 1680 meV | 40 Debye | 23,689 kV/m |

TABLE I. Parameters used in the simulation of the Optical Bloch equations.For simplicity, we assumed equal transition dipole moments for $MoSe_2$ and $WSe_2$.

We simulate two independent two-level systems and a V-Level system, in which the two excited states are coupled together via a common ground state. We also simulated two two-level systems that are coupled together incoherently, which resulted in simulated zero-Quantum spectra practically indistinguishable from its non-coupled counterpart. This allows us to see if we can distinguish between coherent coupling in a V-Level system and chirp-related contributions to two independent two-level systems in the zero-Quantum spectra in the presence of complex chirp.

Since the simulation thus far makes no approximation about the order of the interaction, the resulting solutions would contain all contributions to the polarization from 0th to (technically) infinitely high orders, although lower orders dominate the resulting polarization. In order to filter out contributions detected in our experiment we implement the phase-cycling scheme described in [7], which filters out the same responses that heterodyne detection using lock-in amplifiers, as employed in out setup, does. We exemplarily plot the results of the simulations in Fig. S8 for additional GDD = -1500 $fs^2$ (a), GDD = 0 $fs^2$ (b), and GDD = 1500 $fs^2$ (c). It is evident from these figures that a V-Level and two independent two level systems can be clearly distinguished, despite the influence of chirp. While both system show somewhat of a contribution around the correct mixing energy around -70 meV in Fig. S8 (a), for the two two-level system it is only a weak tail with a maximum at much lower mixing energies and emission energies between the two resonances. For the V-Level system however, there is an emphasized peak around -70 meV, in much better agreement with the experimental results. Moreover, for zero additional GDD, there is a distinct peak at the correct mixing energy for the V-Level system that does not occur for the two two-level systems. Our data shows a peak around -60 meV in this case (see Fig. S7 (b) in the main text). For positive GDD the mixing peak is more pronounced for a V-Level system, but harder to distinguish from two two-level systems than for the negative and zero intentional GDD case. Most notably, our experimental data here shows a clearer peak than the simulation predicts, although some of the spurious contributions at intermediate mixing energies can be obtained when including values down to $T$=0 fs in the experiment, as done in the simulations. All observations considered, it is evident that our data does not match a simple two-level system, but instead resembles the behavior of a V-Level system. The data and simulations for the V-Level system agree well enough, and are distinguished enough from two two-level systems, that we are confident that we are indeed resolving coherent coupling in the heterostructure. We did not fine tune the simulation parameters to get maximum agreement between simulation and data. Rather, the simulation is meant as an illustration that despite complex chirp, a V-Level and two independent two-level systems can be clearly distinguished in a zero-quantum spectrum.

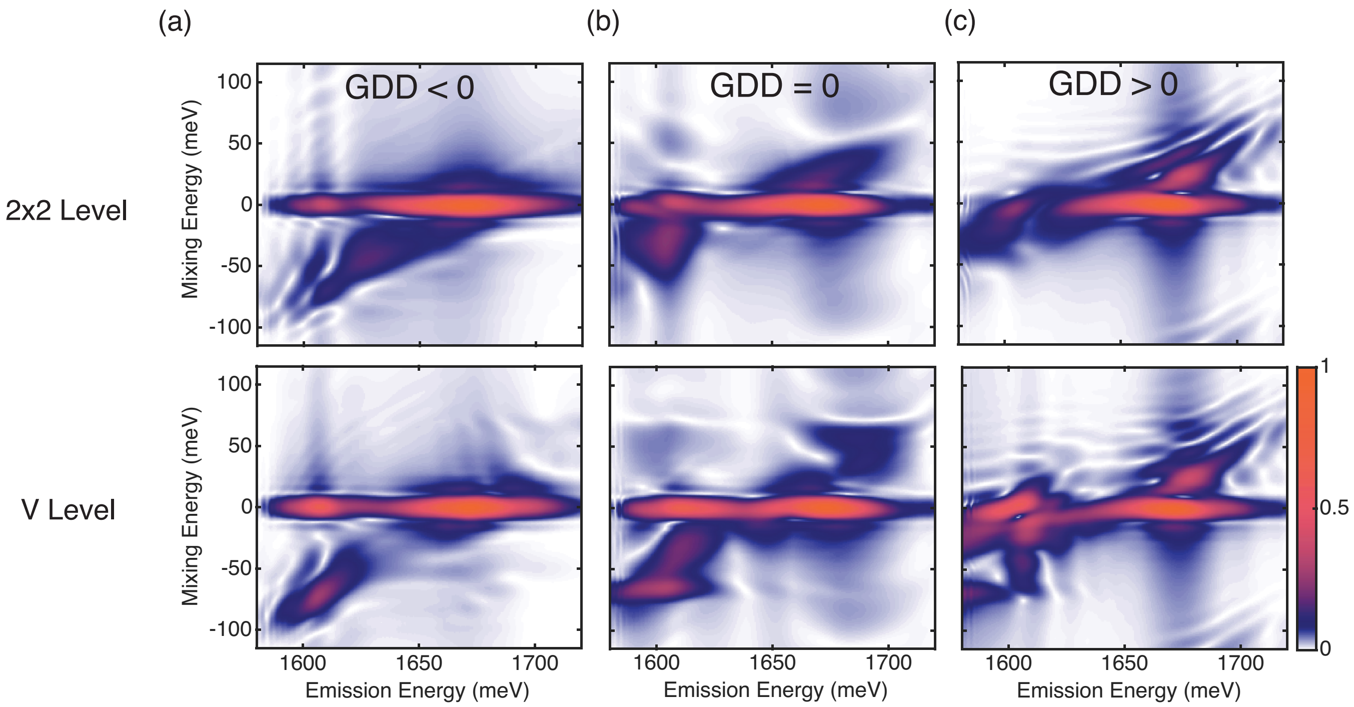


FIG. S8. Optical Bloch Equation simulations of zero-quantum spectra for two independent two level system and a V-Level system in the presence of higher order residual chirp and intentional GDD of -1500 fs$^2$ (a), 0 fs$^2$ (b), and 1500 fs$^2$ (c).

## INTERMEDIATE AND LONG-TERM DYNAMICS

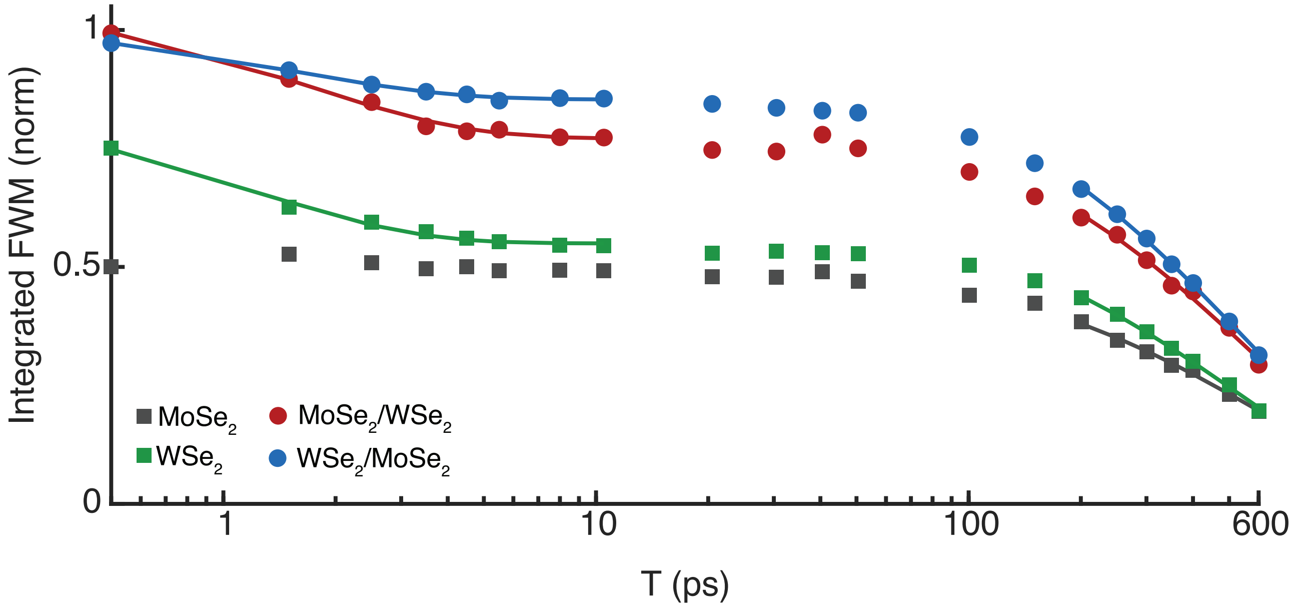


FIG. S9. Complete dataset for intermediate and longterm dynamics from 500 fs to 600 ps.

Omitted in the main text for clarity, we present the complete dataset for intermediate and longterm dynamics in Fig. S9. This data consists of three datasets which were taken separately due to sample drift considerations. The three measurement ranges are 0.5-10.5 ps, 10.5-50.5 ps and 50.5-600.5 ps. Measurements are repeated several times and discarded if sample drift has been observed in between datasets. The dynamics displayed here are the result of

several averaged datasets that have shown no significant sample drift during data taking. The separate time-range measurements are combined by overlapping points between them (10.5 ps and 50.5 ps) and are normalized to the integrated peak amplitudes at $T$=500 fs from the early-time measurement. Also shown are the fits at early and late times, whose results are extensively discussed in the main text. While in the literature often bi-exponential decays are fitted, this is not suitable in this case because of the superposition of different dynamics that we can resolve in MDCS. Since the time scales of the early (fast) and late (slow) decay differ by over two orders of magnitude, it is reasonable to separate the fits into separate exponentials and disregard the intermediate temporal dynamics from 5-100 ps. The fits show good agreement with the data, justifying the model of fitting two separate exponentials.

## SECOND HETEROSTRUCTURE SAMPLE

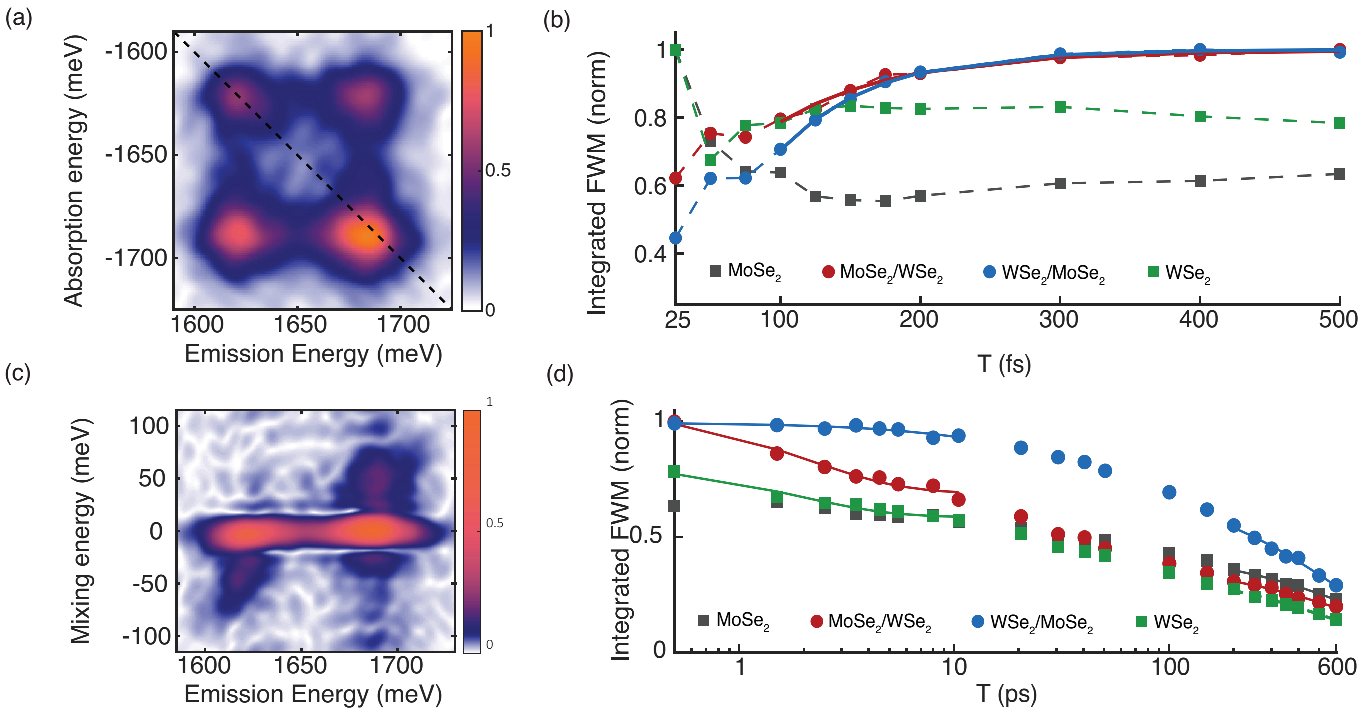


FIG. S10. **a** One-quantum MDCS spectrum at $T$ = 600 fs taken on a similar $MoSe_2/WSe_2$ heterostructure. **b** Early peak dynamics for the sample, showing exponential fits to the rise of the coupling peaks (solid lines) **c** Zero-quantum MDCS spectrum for no intentional GDD **d** Intermediate/longterm peak dynamics with exponential fits (solid lines).

We have also obtained data on a second, similar $MoSe_2/WSe_2$ heterostructure sample, that shows that all the dynamics - the peak rise due to charge transfer, the coherent coupling between the two materials, and any intermediate and longterm dynamics are highly reproducible and not sample specific. In Fig. S10 (a) we show the MDCS spectrum with rephasing and non-rephasing contributions added. Despite adding the two contributions, the four peaks are overall less separated than for the heterostructure presented in the main text. This is partially due to the resonance energy of the $MoSe_2$ being roughly 15 meV higher in this material, and partially due to the fact that the $MoSe_2$ peak is significantly broader. While the absolute time-scales differ, it is evident from Fig. S10 (b) that the dynamics agree with the other heterostructure qualitatively: We see a rapid decay of the on-diagonal peaks, accompanied by a rapid rise for the two coupling peaks. Note that the broader linewidths correlate with faster charge transfer (67 fs from $WSe_2$ to $MoSe_2$ and 85 fs from $MoSe_2$ to $WSe_2$), supporting the statement in the main text that the new dephasing channels are significantly influenced by population decay due to charge transfer. We also again see a signature of coherent coupling at early times, with non-zero amplitudes for the coupling peaks and residual oscillations, which can be supported by the zero-quantum spectrum in Fig. S10 (c). This zero-quantum spectrum was taken at zero additional GDD and the center of the zero-quantum peaks is thus slightly lower than the 55 meV energy difference between the resonances in the two materials. The intermediate and longterm dynamics in Fig. S10 (d) also show a behavior very similar to the one observed for the heterostructure discussed in the main text. At intermediate times, the $WSe_2$ peak and the $MoSe_2/WSe_2$ see a significant decay while the $WSe_2/MoSe_2$ peak barely decays and the $MoSe_2$ peak rises.

Again, the peaks decay at longer time-scales ($891 \pm 36$ ps, $861 \pm 55$ ps, $634 \pm 35$ ps ,$615 \pm 30$ ps from left to right, top to bottom) which we again attribute to the interlayer exciton relaxation.

[1] M. E. Siemens, G. Moody, H. Li, A. D. Bristow, and S. T. Cundiff, Resonance lineshapes in two-dimensional faourier transform spectroscopy, Opt. Express **18**, 17699 (2010).

[2] E. W. Martin, J. Horng, H. G. Ruth, E. Paik, M.-H. Wentzel, H. Deng, and S. T. Cundiff, Encapsulation narrows and preserves the excitonic homogeneous linewidth of exfoliated monolayer $MoSe_2$, Phys. Rev. Applied **14**, 021002 (2020).

[3] G. Moody, C. Kavir Dass, and K. e. a. Hao, Intrinsic homogeneous linewidth and broadening mechanisms of excitons in monolayer transition metal dichalcogenides, Nat Commun **6**, 8315 (2015).

[4] D. Polli, D. Brida, S. Mukamel, G. Lanzani, and G. Cerullo, Effective temporal resolution in pump-probe spectroscopy with strongly chirped pulses, Phys. Rev. A **82**, 053809 (2010).

[5] X. Hong, J. Kim, and S. e. a. Shi, Ultrafast charge transfer in atomically thin mos2/ws2 heterostructures, Nature Nanotech , 682–686 (2014).

[6] G. Moody and S. T. Cundiff, Advances in multi-dimensional coherent spectroscopy of semiconductor nanostructures, Advances in Physics: X **2**, 641 (2017), pMID: 28894306, https://doi.org/10.1080/23746149.2017.1346482.

[7] P. Tian, D. Keusters, Y. Suzaki, and W. S. Warren, Femtosecond phase-coherent two-dimensional spectroscopy, Science **300**, 1553 (2003), https://science.sciencemag.org/content/300/5625/1553.full.pdf.
